# Supplementary material for: DyTed: Disentangled Representation Learning for Discrete-time Dynamic Graph
Source: arXiv:2210.10592 source file (2023-08-16)
Supplement: Supplementary file 1 [file 7-appendix-ablation.tex]

\begin{table}
  \centering
  \caption{Ablation Study}
  \resizebox{3.4in}{!}{
  \begin{threeparttable}
    \begin{tabular}{lccccc}
    \toprule
    \textbf{Model} & \textbf{Uci} &\textbf{Bitcoin} &\textbf{As722} &\textbf{HepTh} &\textbf{HepPh} \\
    \midrule
    \textbf{LSTMGCN-DyTed}                            & $\bm{76.06}$ & $\bm{79.02}$ & $\bm{81.82}$ & $\bm{85.88}$ & $\bm{87.12}$   \\
    \hspace{0.3cm}-Random Sampling                    & $71.09$ & $77.72$ & $80.57$ & $85.79$ & $87.03$\\
    \hspace{0.3cm}-w/o Time-varying Generator         & $72.85$ & $69.83$ & $73.69$ & $76.49$ & $82.78$\\
    \hspace{0.3cm}-w/o Discriminator                  & $76.03$ & $76.88$ & $80.52$ & $85.58$ & $86.12$  \\
    \midrule
    \specialrule{0em}{0.5pt}{0.5pt}
    \midrule
    \textbf{DySAT-DyTed}                              & $\bm{86.12}$ & $\bm{83.32}$ & $\bm{84.47}$ & $\bm{80.76}$ & $\bm{78.68}$   \\
    \hspace{0.3cm}-Random Sampling                    & $74.24$ & $82.91$ & $83.04$ & $79.26$ & $75.69$ \\
    \hspace{0.3cm}-w/o Time-varying Generator         & $71.26$ & $79.61$ & $78.7$ & $74.87$ & $71.66$ \\
    \hspace{0.3cm}-w/o Discriminator                  & $78.20$ & $80.21$ & $84.38$ & $77.47$ & $76.01$  \\
    \midrule
    \specialrule{0em}{0.5pt}{0.5pt}
    \midrule
    \textbf{HTGN-DyTed}                               & $\bm{92.08}$ & $\bm{84.56}$ & $\bm{77.08}$ & $\bm{75.61}$ & $\bm{74.46}$  \\
    \hspace{0.3cm}-Random Sampling                    & $85.09$ & $82.21$ & $76.00$ & $73.05$ & $74.26$\\
    \hspace{0.3cm}-w/o Time-varying Generator         & $85.73$ & $70.54$ & $76.92$ & $73.81$ & $73.85$\\
    \hspace{0.3cm}-w/o Discriminator                  & $90.93$ & $84.01$ & $77.01$ & $72.31$ & $74.21$ \\
    \midrule
    \specialrule{0em}{0.5pt}{0.5pt}
    \midrule
    \textbf{ROLAND-DyTed}                            & $\bm{88.05}$ & $\bm{88.59}$ & $\bm{76.96}$ & $\bm{81.14}$ & $\bm{80.50}$\\
    \hspace{0.3cm}-Random Sampling                   & $84.11$ & $86.32$ & $74.89$ & $78.11$ & $79.19$ \\
    \hspace{0.3cm}-w/o Time-varying Generator        & $73.97$ & $86.95$ & $74.83$ & $78.72$ & $79.87$\\
    \hspace{0.3cm}-w/o Discriminator                 & $85.76$ & $84.34$ & $74.16$ & $80.47$ & $80.10$ \\
    \bottomrule
    \end{tabular}%
    \end{threeparttable}
    }
  \label{tab:appendix_ab}%
\end{table}%
